# Supplementary material for: SABER-6D: Shape Representation Based Implicit Object Pose Estimation
Source: arXiv:2408.05867 source file (2024-09-02)
Supplement: Supplementary file 1 [file X_suppl.tex]

% \clearpage
% \setcounter{page}{1}

\title{Supplementary Material \\ Alignist: CAD-Informed Orientation Distribution Estimation by Fusing Shape and Correspondences }
\maketitle 

We present training details, and additional quantitative and qualitative results in the following sections.
\section{Training Details}
\subsection{Network Architecture}
We employ a ResNet50 encoder similar to other approaches, IPDF\cite{esteves2021generalized}, SpyroPose\cite{haugaard2023spyropose}, and Normalizing Flow\cite{liu2023delving}. We employ two 4-layer MLPs with ReLU activations with 256 dimensional hidden layers each for predicting SDF probability and feat probability. Cube positional encoding comprises encoding transformed vertices of a cube with a rotation matrix. The positional encoding is applied on eight 3D vertices of the cube with 3 frequencies and concatenated to create a 144-dimensional embedding to represent the rotation matrix. The encoder takes the image and predicts a 2048-dimensional image embedding. We employ two linear layers to convert rotation embedding and image embedding to 256 dimensional embeddings which are then added and passed through two MLPs to predict the probabilities. Symsol dataset doesn't provide CAD models. It was easier to get models for Symsol-I as they are readily available in any 3D library and are canonically aligned with the dataset. For Symsol-II, we employed differentiable rendering initially using silhouettes to estimate camera intrinsics because the shapes were canonically aligned. We employ differentiable rendering to transfer texture from images to the CAD models using the learned intrinsics and the rotation labels. 

\subsection{SurfEmb Network}
We follow the default configuration provided in SurfEmb\cite{haugaard2022surfemb} and train using PBR-rendered data from the CAD models for 100k iterations. We extract the SurfEmb feature MLP which is employed in our pipeline to estimate feature based probability. SurfEmb Feature MLP employs a 4-layer Siren MLP which takes a single 3D point and predicts the corresponding feature vector.

\subsection{SDF Network}
We employ a 4-layer Siren MLP with 256 dimensional hidden layers which takes a single 3D point and predicts the corresponding SDF value. We randomly generate 3D points and estimate SDF values for those 3D points using the CAD model. The 3D points and SDF values are used for training the SDF network which remembers the CAD model implicitly by learning SDF values for 3D points. 

\subsection{Training}
We render a NOCS image for every input image using the CAD model and rotation label. We sample 100 pixels inside the mask to extract a 3D point cloud with 100 points. We rotate this with the inverse of ground truth rotation to get the image-aligned point cloud. We employ 4096 rotations to pair with each image to learn the distribution for that specific image. We sample 3000 rotations from the top 20000 rotations in the precomputed distribution. We sample 1095 rotations randomly from a uniform distribution. We also add the ground truth rotation in the employed rotations. We can precompute the scores for every image before the start of training or we can compute them online. We prefer to compute them online so that we can sample randomly without getting restricted to a grid. For each rotation, we compute both SDF probability and feature probability and use them as supervision for probabilities predicted from the network. We employed a batch size of 128 for the network to train on the Symsol dataset and 64 for the T-Less dataset and ModelNet10-SO3. 

\subsection{Mode Focused Sampling}

For each image, we sample 4K rotations to learn the pose distribution. Since we can precompute the distribution for a given training image, we can sample more rotation matrices near the modes to learn a much sharper distribution. Mode focused sampling helps in learning sharper distribution which is possible because of the precomputable distribution from CAD model through SurfEmb features and SDF based shape networks.

% \section{Positional Encoding with IPDF}
% In the main paper, we presented the impact of cube positional encoding (cube PE) on our approach compared to the positional encoding proposed in IPDF. We evaluate IPDF approach using IPDF positional encoding and our positional encoding to see the impact of the proposed positional encoding on the IPDF approach. We observe that cube PE performs better than IPDF PE by an increase in log-likelihood of 1.01. 

\section{ Additional Quantitative results}
\subsection{ModelNet-SO3}
We perform experiments on ModelNet-SO3 to understand the category level generalization capabilities of our approach. ModelNet-SO3 comprises 10 categories which contain synthetic renderings of around 100 CAD models for each category as the training set. The test set comprises synthetic renderings of unseen instances of the same categories. We choose a single CAD model per category which acts as a 3D representation of the category for training our Shape and Feature experts. During training, we employ distribution supervision from the chosen single CAD model per category. While we employ images from all the provided synthetic renderings, the distribution supervision comes from the chosen CAD model. Ideally, we would employ the same CAD model as the instance present in the image, but it is difficult to train SurfEmb and SDF networks for so many CAD models. Despite using distribution supervision from a single CAD model per category, we achieve closer to the benchmark approaches, NF and IPDF. We trained a separate model per category and presented the results in Table \ref{tab:modelnet}. 

\begin{table}[!t]\centering

\caption{Evaluations on ModelNet-SO3.}
% \small
% \tabcolsep=0.225cm
\begin{tabular}{l|ccc}
Metric &IPDF &NF &Ours \\
\midrule
$AR@30^{\circ}$&  0.735 & 0.774 & 0.705 \\
% ModelNet10-SO3 &AR@$30^\circ$ &92.50 &\textbf{94.20} &92.10 \\

% \bottomrule
\end{tabular}\label{tab:modelnet}

\end{table}

\subsection{T-Less BOP}
We evaluate IPDF, our approach, and NF on T-less scenes with occlusions by training on synthetic PBR data from the BOP challenge rendered from CAD models. We trained both our approach and NF for 100k iterations. We achieve better log-likelihood compared to NF as shown in in Table \ref{tab:tless-real}. Note that we only trained and evaluated using allocentric rotation representation and ignored translation component. 

\begin{table}[!t]\centering

\caption{Evaluations on occluded real scenes of T-Less BOP using the Log-Likelihood (LL) trained for 100k iterations.}
% \small
% \tabcolsep=0.225cm
\begin{tabular}{l|ccc}
Metric &IPDF &NF &Ours \\
\midrule
LL& 5.31&6.23 &\textbf{6.64} \\
% ModelNet10-SO3 &AR@$30^\circ$ &92.50 &\textbf{94.20} &92.10 \\

% \bottomrule
\end{tabular}\label{tab:tless-real}

\end{table}
\subsection{Spread on SYMSOL-I}
Spread measures the expected angular deviation from all ground truth symmetric annotations which measures the angular deviation and uncertainty around them. We present spread results on SYMSOL-I dataset in Table \ref{tab:spread}. WE observe that we have lower spread compared to NF at 100k while NF performs better than us after 900k iterations.  
\begin{table}[!t]\centering
\caption{Spread on Symsol-I dataset in degrees. Spread measures the expectation of median angular error over all the ground truth rotations. NF-100k, NF-900k refers to Normalizing flow trained for 100k and 900k iterations respectively. 
% \tolga{What is spread? Why is lower the better?}
}\label{tab:spread}
\scriptsize
\begin{tabular}{lrrrrr}

Spread &Deng &IPDF &NF-100k &NF-900k &Ours \\\midrule
cone &10.1 &1.4 &0.9 &0.5 &0.5 \\
cube &40.7 &4.0 &2.0 &0.6 &0.6 \\
cyl &15.2 &1.4 &0.9 &0.5 &0.5 \\
icosa &29.5 &8.4 &9.2 &1.1 &3.5 \\
tet &16.7 &4.6 &1.7 &0.6 &1.0 \\\hline
avg &22.4 &4.0 &2.9 &\textbf{0.7} &1.4 \\

\end{tabular}
\end{table}

\subsection{Performance on SYMSOL-II}
Our LL on SYMSOL-II is impacted by a domain gap as we had to texture the CAD models using differentiable rendering of images. Moreover, LL in SYMSOL-II considers only a single valid mode(the pose the image is rendered) for evaluation even though there are multiple valid modes. This contrasts with SYMSOL-I, where all valid modes are evaluated. Additionally, LL metric inherently favors NF since NF can provide exact LL estimation. In contrast, both IPDF and our approach evaluate LL on a discrete grid of rotations, making our methods limited by finite resolution.
% \subsection{Low-Data plot}
% To show the efficiency of our approach in low-data regime, we plot the Log-Likelihood vs training data plot in Figure \ref{fig:dataplot}. The gap between the Log-Likelihoods attained by our method and those by Normalizing Flow (NF) increases rapidly as the amount of training data decreases. This shows that the presence of CAD model can help learn about symmetries    
% \begin{figure}
% \centering
% \includegraphics[width=0.5\textwidth]{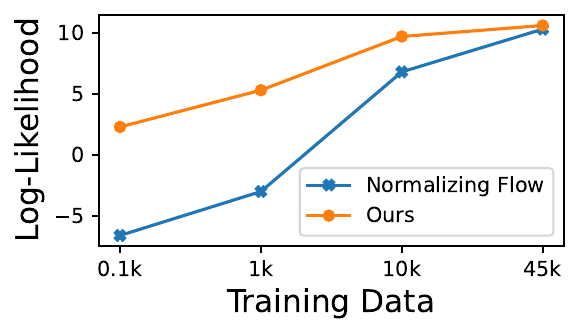}
% \caption{\small\label{fig:dataplot}Log-Likelihood vs. Training Data for NF and Ours on SYMSOL-I.\vspace{-4mm}
% }
% \end{figure}

\section{Efficiency} Inferring rotation distributions takes 10ms at a grid of 2 million rotations on NVIDIA Titan X. NF takes 210ms for rotation estimation, but longer to construct the distribution as the full base distribution is mapped onto the target.

\section{Qualitative results}
We present more distribution visualization results for all objects in the Symsol dataset. We follow the IPDF approach to visualize the top-k probabilities on a 2D sphere where each point on the sphere represents an axis of rotation and the color of the point indicates the tilt about that axis. We visualize distribution on Symsol-I and Symsol-II as described in IPDF in Figures \ref{fig:SymsolViz1} and \ref{fig:SupSymsol2Viz} respectively. We also visualize the SurfEmb features of tetX object in \ref{fig:featViz}. We also visualize distribution by rotating coordinate reference frames with top-k rotations and projecting them on the image as shown in Figure \ref{fig:ourViz}. 

\begin{figure}
     \centering
     \begin{subfigure}{.3\linewidth}
     \centering
     \includegraphics[width=1\textwidth]{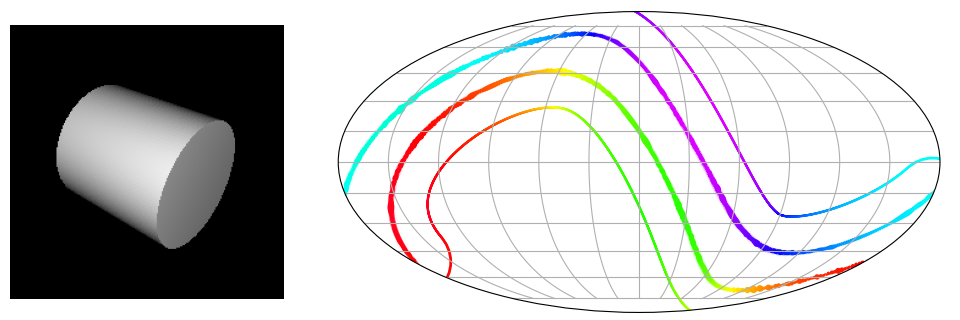}
     % \caption{Cyl-Symsol-I\label{fig:dcyl1}}
     \end{subfigure}%
     \hfill
     \begin{subfigure}{.3\linewidth}
     \centering
     \includegraphics[width=1.\textwidth]{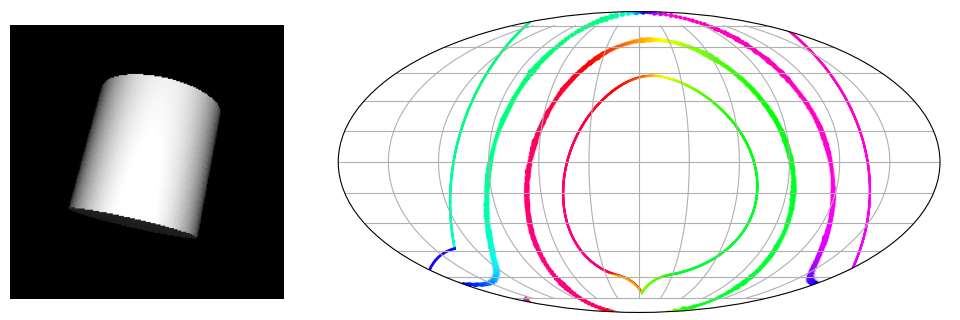}
     % \caption{Cyl-Symsol-I\label{fig:dcyl2}}
     \end{subfigure}%
     \hfill
     \begin{subfigure}{.3\linewidth}
     \centering
     \includegraphics[width=1\textwidth]{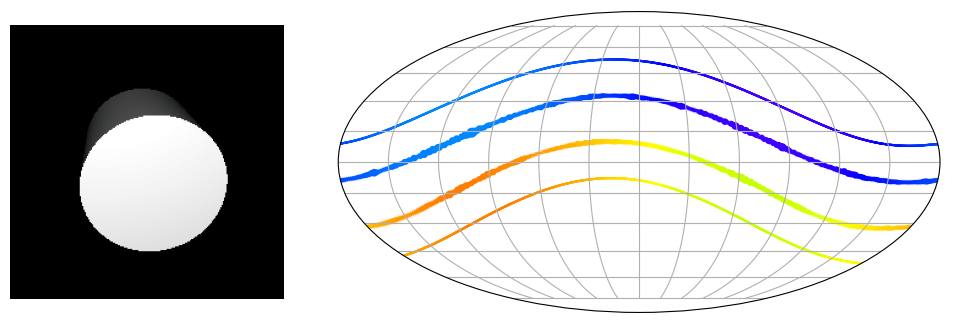}
     % \caption{Cyl-Symsol-I\label{fig:dcyl3}}
     \end{subfigure}%
     \hfill
     \\
     \begin{subfigure}{.3\linewidth}
     \centering
     \includegraphics[width=1\textwidth]{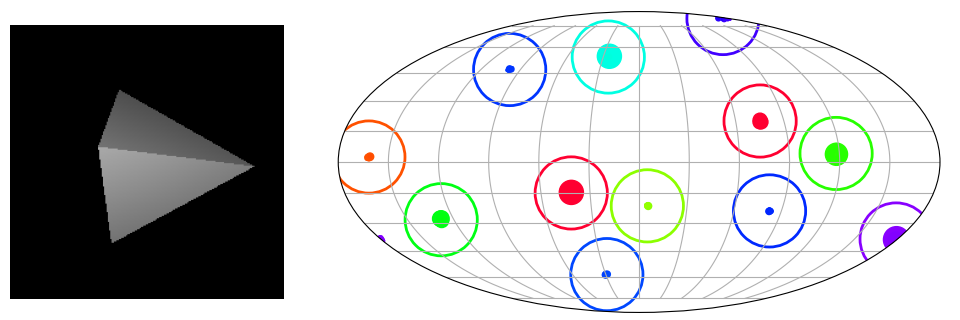}
     % \caption{Tet-Symsol-I\label{fig:tetS1}}
     \end{subfigure}%
     \hfill
     \begin{subfigure}{.3\linewidth}
     \centering
     \includegraphics[width=1.\textwidth]{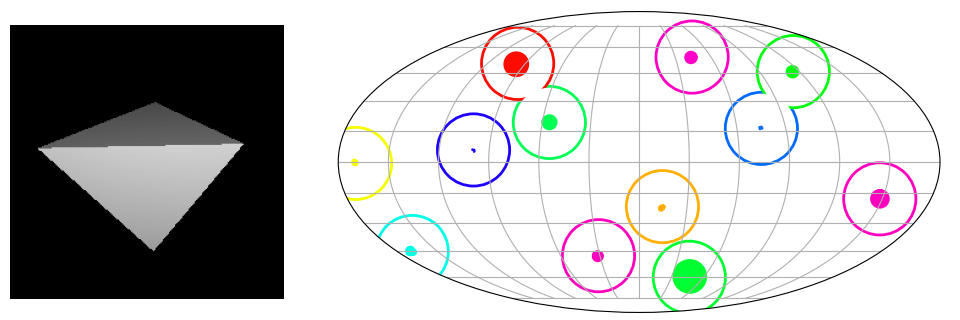}
     % \caption{Tet-Symsol-I\label{fig:tetS2}}
     \end{subfigure}%
     \hfill
     \begin{subfigure}{.3\linewidth}
     \centering
     \includegraphics[width=1\textwidth]{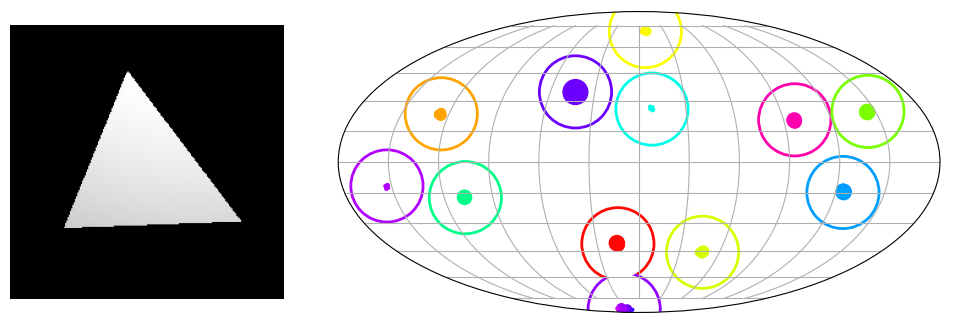}
     % \caption{Tet-Symsol-I\label{fig:tet2S2}}
     \end{subfigure}%
     \hfill
     \\
     \begin{subfigure}{.3\linewidth}
     \centering
     \includegraphics[width=1\textwidth]{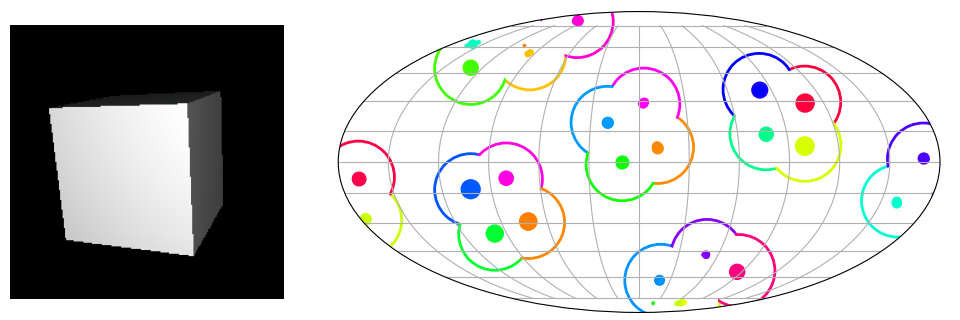}
     % \caption{Cube-Symsol-I\label{fig:tetS1}}
     \end{subfigure}%
     \hfill
     \begin{subfigure}{.3\linewidth}
     \centering
     \includegraphics[width=1.\textwidth]{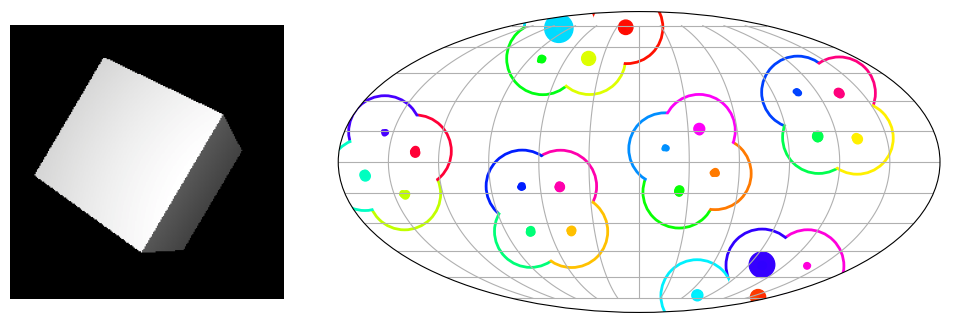}
     % \caption{Cube-Symsol-I\label{fig:tetS2}}
     \end{subfigure}%
     \hfill
     \begin{subfigure}{.3\linewidth}
     \centering
     \includegraphics[width=1\textwidth]{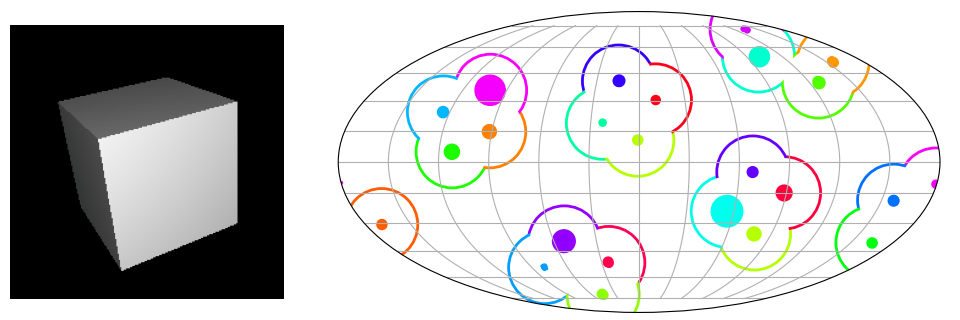}
     % \caption{Cube-Symsol-I\label{fig:tet2S2}}
     \end{subfigure}%
     \hfill
      \\
     \begin{subfigure}{.3\linewidth}
     \centering
     \includegraphics[width=1\textwidth]{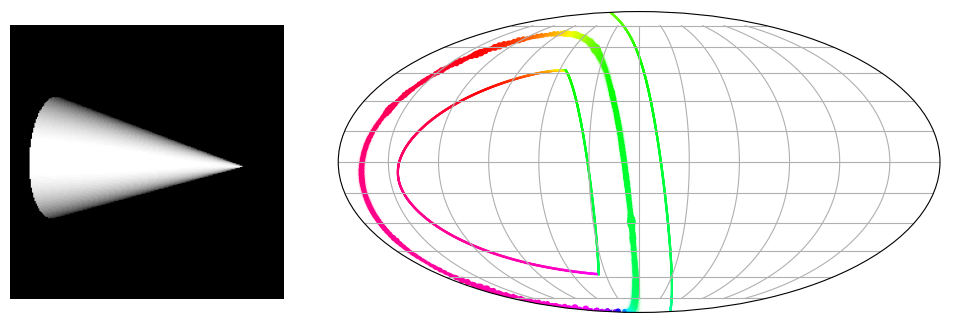}
     % \caption{Cone-Symsol-I\label{fig:tetS1}}
     \end{subfigure}%
     \hfill
     \begin{subfigure}{.3\linewidth}
     \centering
     \includegraphics[width=1.\textwidth]{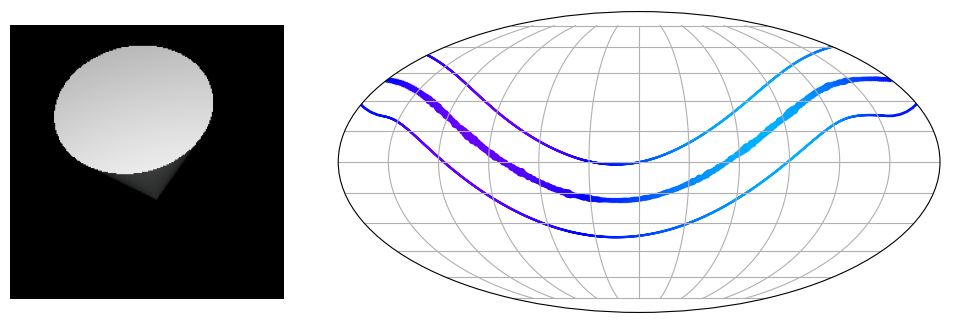}
     % \caption{Cone-Symsol-I\label{fig:tetS2}}
     \end{subfigure}%
     \hfill
     \begin{subfigure}{.3\linewidth}
     \centering
     \includegraphics[width=1\textwidth]{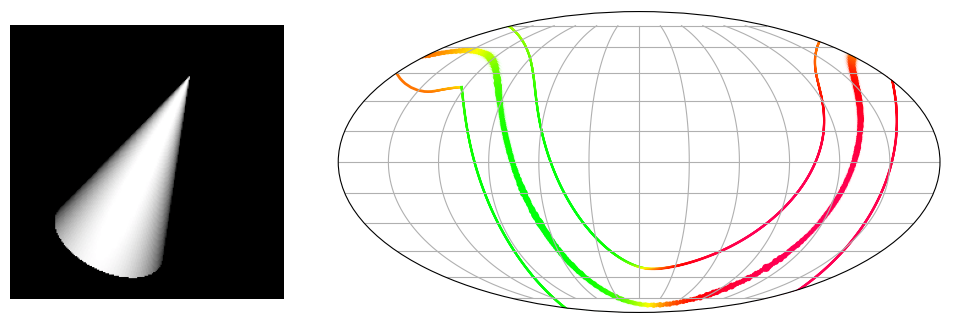}
     % \caption{Cone-Symsol-I\label{fig:tet2S2}}
     \end{subfigure}%
     \hfill
     %  \\
     % \begin{subfigure}{.3\linewidth}
     % \centering
     % \includegraphics[width=1\textwidth]{images/distImages/tet_00126.png}
     % % \caption{Tet-Symsol-I\label{fig:tetS1}}
     % \end{subfigure}%
     % \hfill
     % \begin{subfigure}{.3\linewidth}
     % \centering
     % \includegraphics[width=1.\textwidth]{images/distImages/tet_00736.png}
     % % \caption{Tet-Symsol-I\label{fig:tetS2}}
     % \end{subfigure}%
     % \hfill
     % \begin{subfigure}{.3\linewidth}
     % \centering
     % \includegraphics[width=1\textwidth]{images/distImages/tet_01048.png}
     % % \caption{Tet-Symsol-I\label{fig:tet2S2}}
     % \end{subfigure}%
     % \hfill
     %
         % \includegraphics[width=0.19\textwidth]{sources/images/alignedbadly2.PNG}
      
     \caption{Pose distribution visualization for different objects in Symsol-I. Each row corresponds to a single object from Symsol. The distributions for cylinder, tetrahedron, cube, and cone objects are visualized. Cylinder and cone express continuous symmetries indicated by smooth curves, unlike tetrahedron and cube which have discrete modes.        
     \vspace{-4mm}
     }
     \label{fig:SymsolViz1}
\end{figure}
\begin{figure}
     \centering
     \begin{subfigure}{.3\linewidth}
     \centering
     \includegraphics[width=1\textwidth]{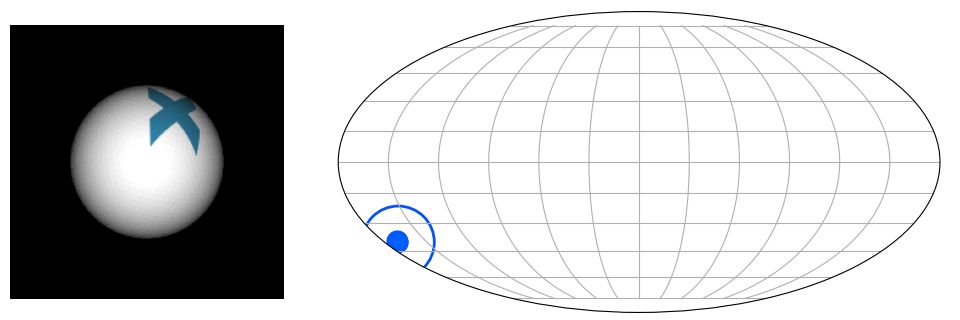}
     % \caption{Cyl-Symsol-I\label{fig:dcyl1}}
     \end{subfigure}%
     \hfill
     \begin{subfigure}{.3\linewidth}
     \centering
     \includegraphics[width=1.\textwidth]{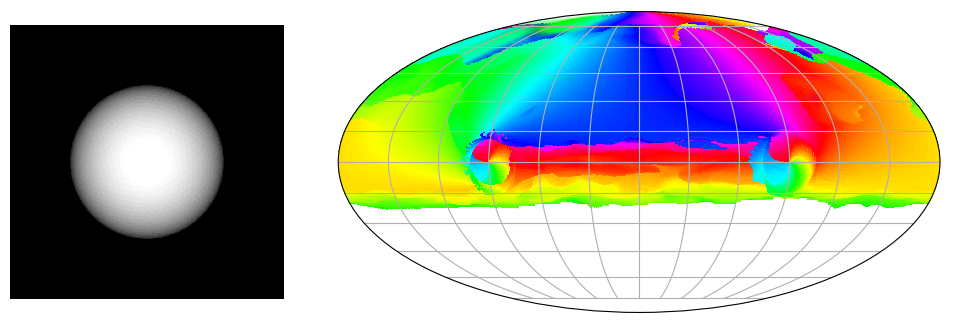}
     % \caption{Cyl-Symsol-I\label{fig:dcyl2}}
     \end{subfigure}%
     \hfill
     \begin{subfigure}{.3\linewidth}
     \centering
     \includegraphics[width=1\textwidth]{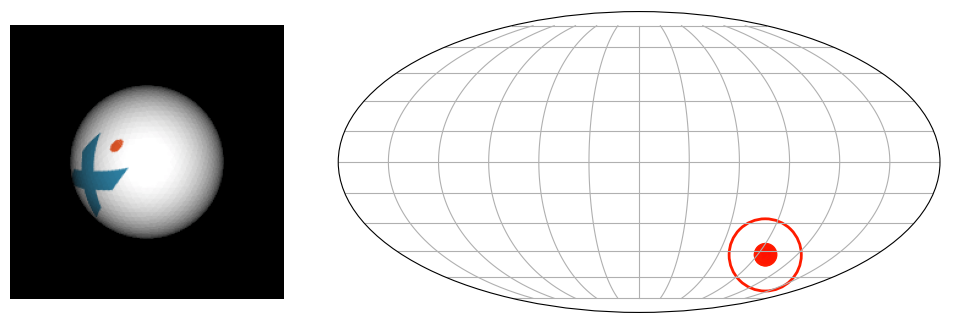}
     % \caption{Cyl-Symsol-I\label{fig:dcyl3}}
     \end{subfigure}%
     \hfill
     \\
     \begin{subfigure}{.3\linewidth}
     \centering
     \includegraphics[width=1\textwidth]{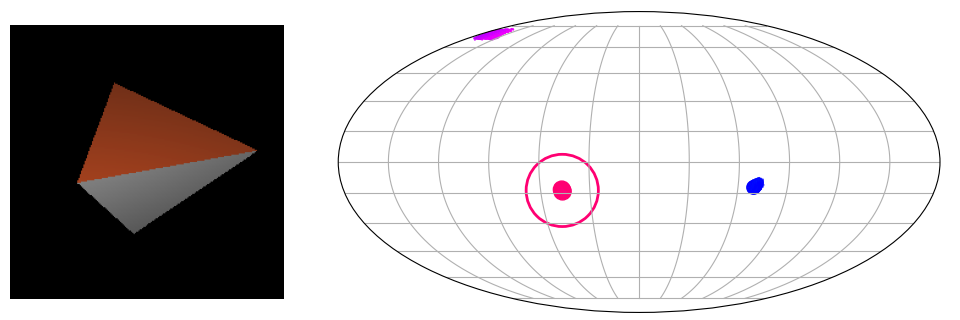}
     % \caption{Tet-Symsol-I\label{fig:tetS1}}
     \end{subfigure}%
     \hfill
     \begin{subfigure}{.3\linewidth}
     \centering
     \includegraphics[width=1.\textwidth]{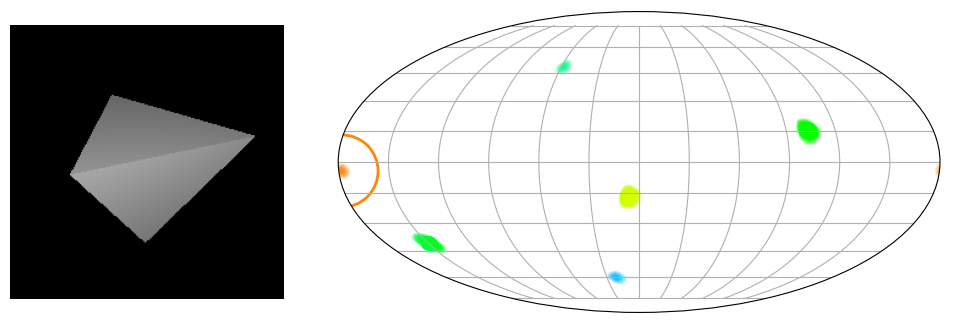}
     % \caption{Tet-Symsol-I\label{fig:tetS2}}
     \end{subfigure}%
     \hfill
     \begin{subfigure}{.3\linewidth}
     \centering
     \includegraphics[width=1\textwidth]{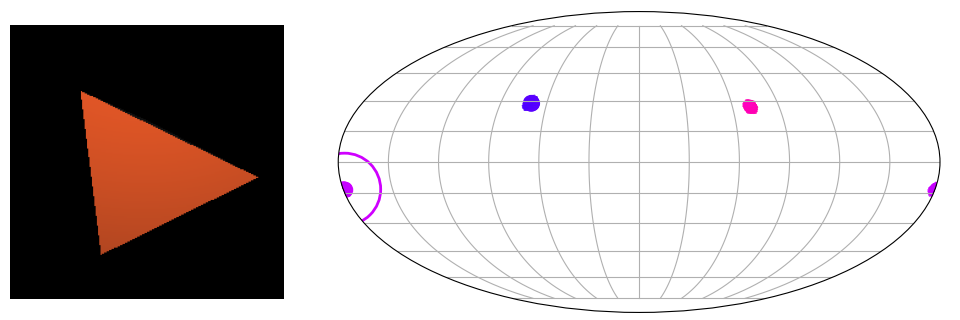}
     % \caption{Tet-Symsol-I\label{fig:tet2S2}}
     \end{subfigure}%
     \hfill
     \\
     \begin{subfigure}{.3\linewidth}
     \centering
     \includegraphics[width=1\textwidth]{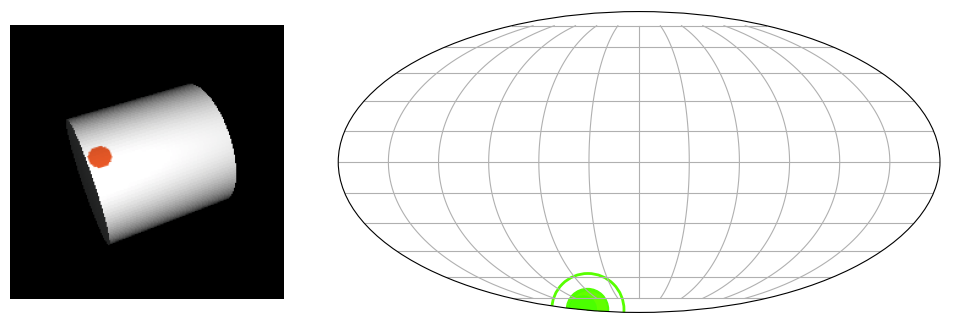}
     % \caption{Cube-Symsol-I\label{fig:tetS1}}
     \end{subfigure}%
     \hfill
     \begin{subfigure}{.3\linewidth}
     \centering
     \includegraphics[width=1.\textwidth]{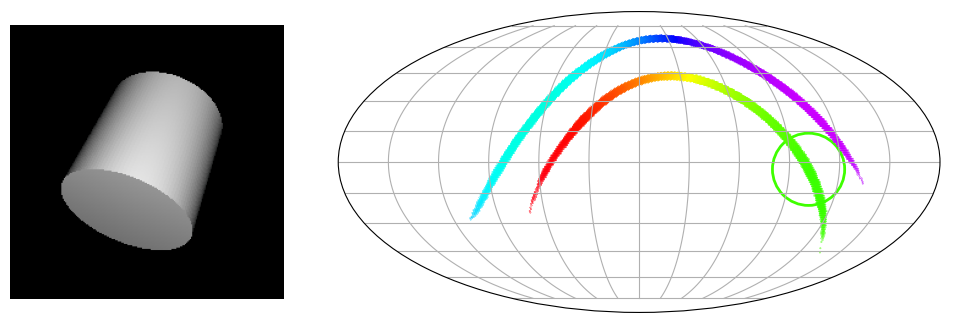}
     % \caption{Cube-Symsol-I\label{fig:tetS2}}
     \end{subfigure}%
     \hfill
     \begin{subfigure}{.3\linewidth}
     \centering
     \includegraphics[width=1\textwidth]{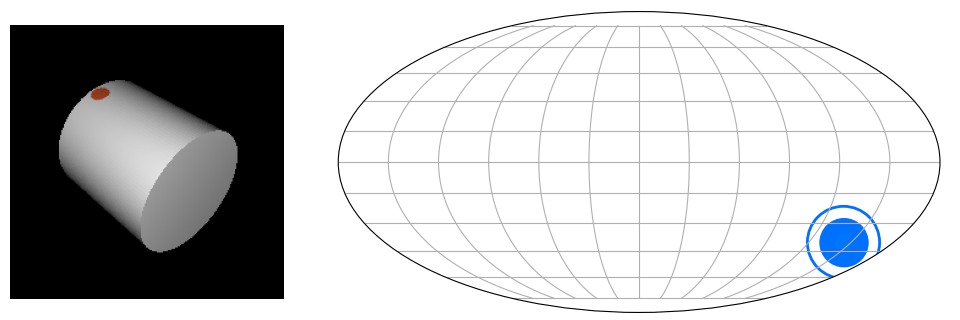}
     % \caption{Cube-Symsol-I\label{fig:tet2S2}}
     \end{subfigure}%
     \hfill
     \caption{Pose distribution visualization for different objects in Symsol-II. Each row corresponds to images from SphereX, TetX and CylO objects respectively. The middle column indicates the distribution when the markers are not visible. The left and right columns indicate the sharper distribution when the markers are visible. This shows that our approach can capture the distribution based on the texture component and make it sharper based on the marker when it is visible. This is possible because of the surfemb features which learn different features for textured regions and different features for untextured regions as shown in Figure \ref{fig:featViz}.
     \label{fig:SupSymsol2Viz}}
\end{figure}

\begin{figure}
     \centering
     \begin{subfigure}{.5\linewidth}
     \centering
     \includegraphics[width=1\textwidth]{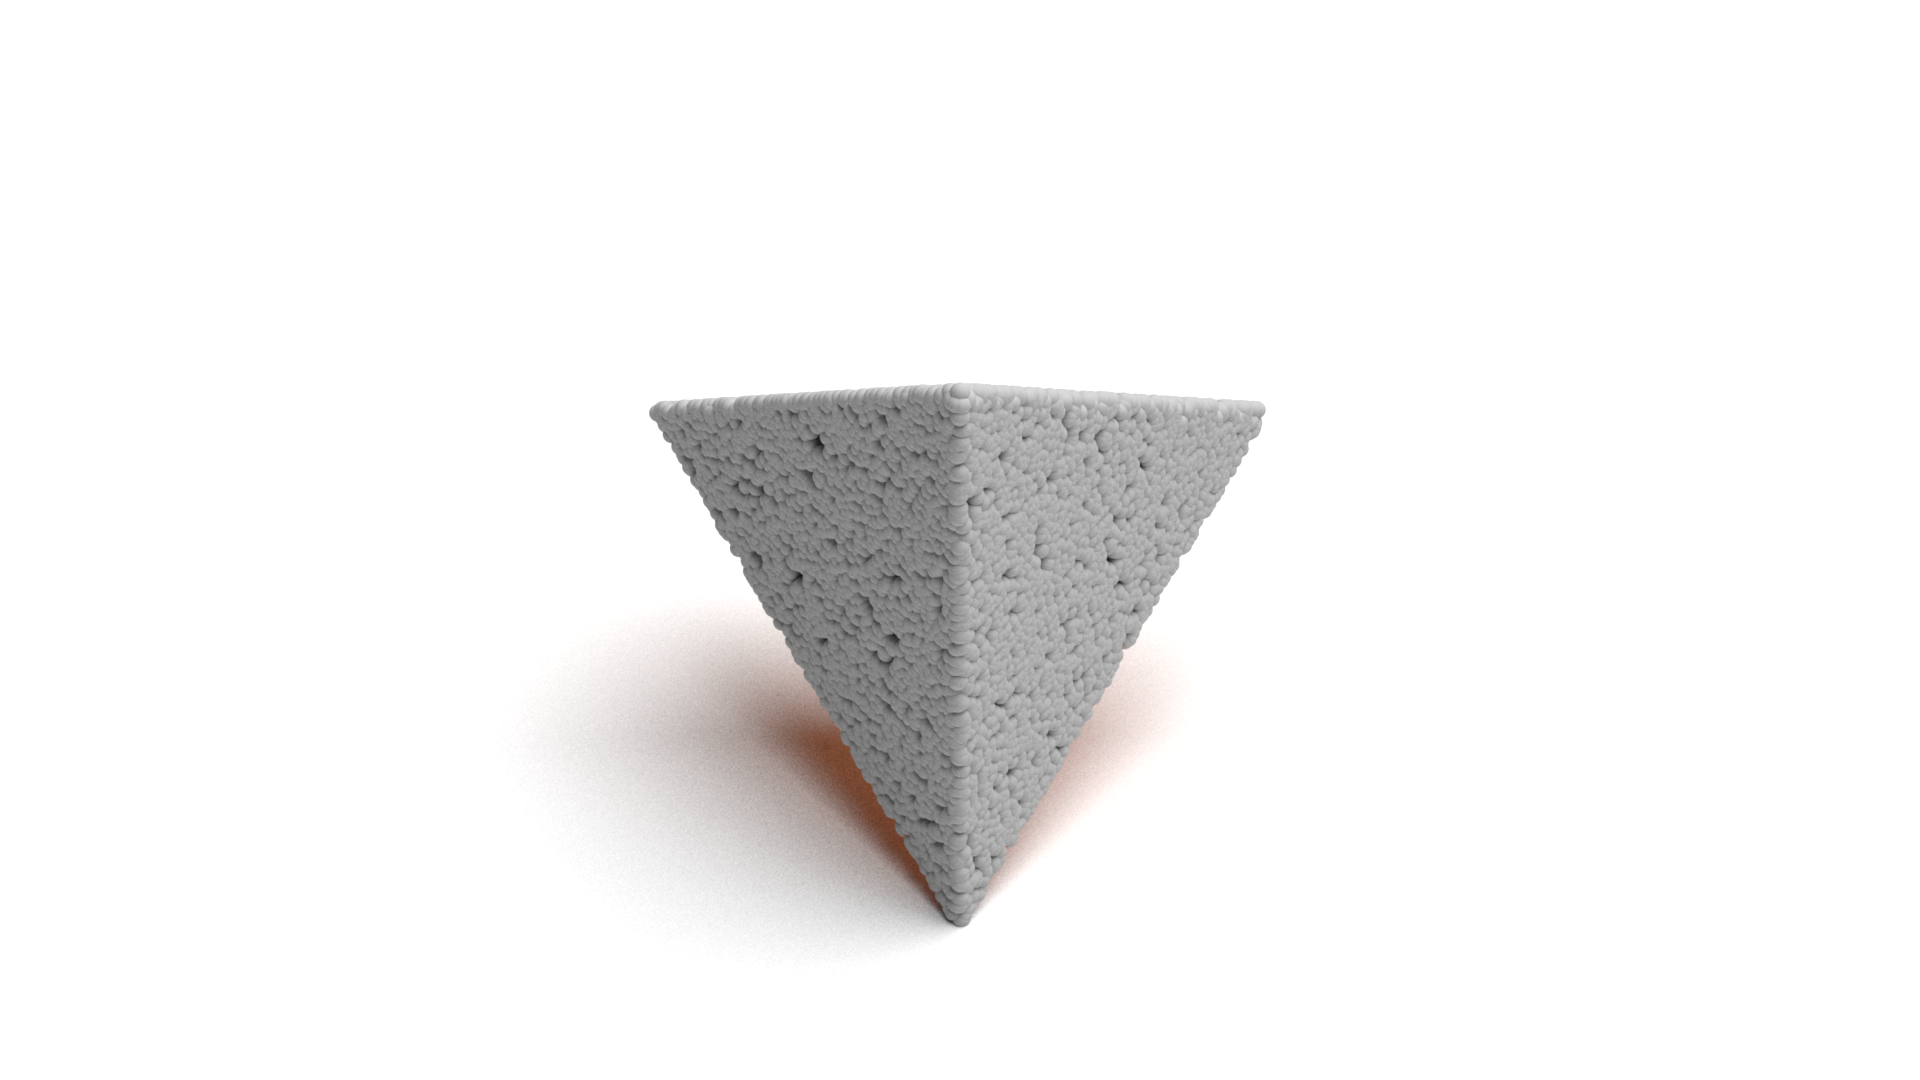}
     % \caption{Cyl-Symsol-I\label{fig:dcyl1}}
     \end{subfigure}%
     \hfill
     \begin{subfigure}{.5\linewidth}
     \centering
     \includegraphics[width=1.\textwidth]{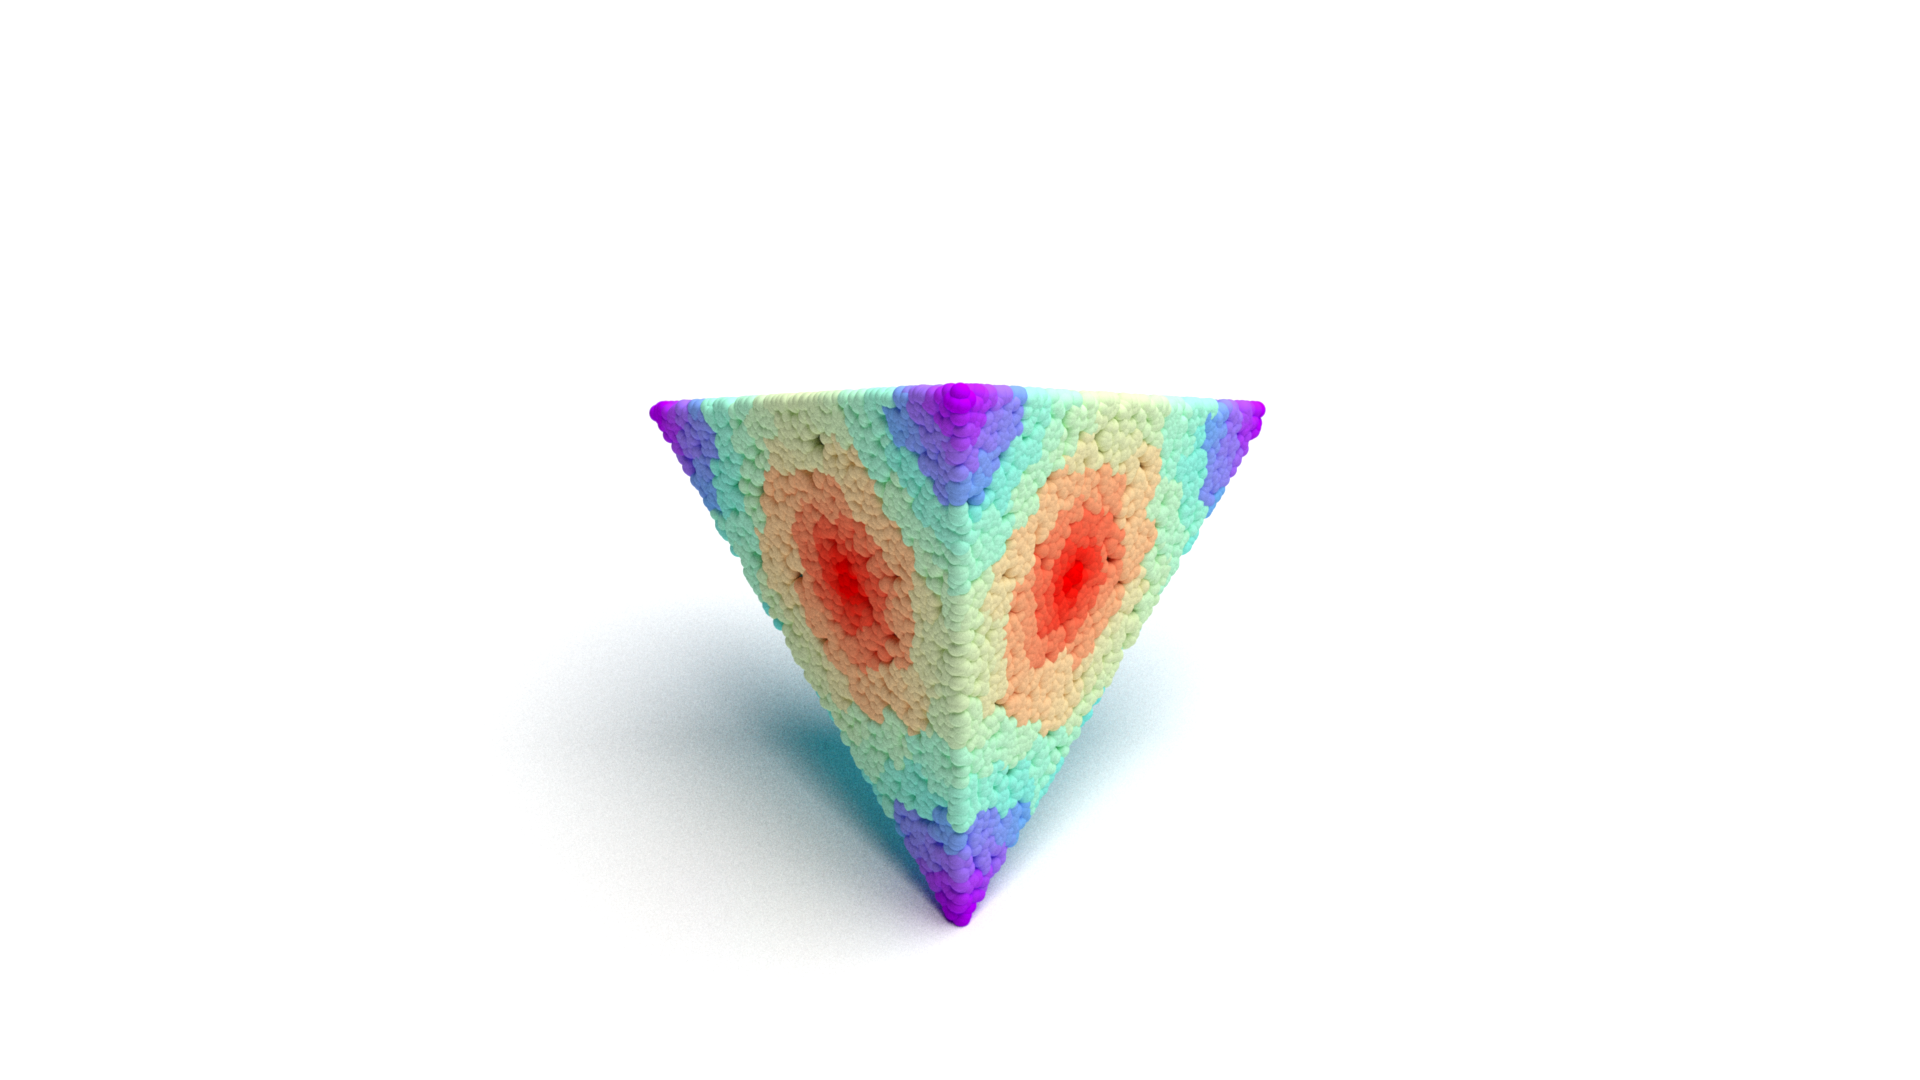}
     % \caption{Cyl-Symsol-I\label{fig:dcyl2}}
     \end{subfigure}%
     \hfill
     \\
     \begin{subfigure}{.5\linewidth}
     \centering
     \includegraphics[width=1\textwidth]{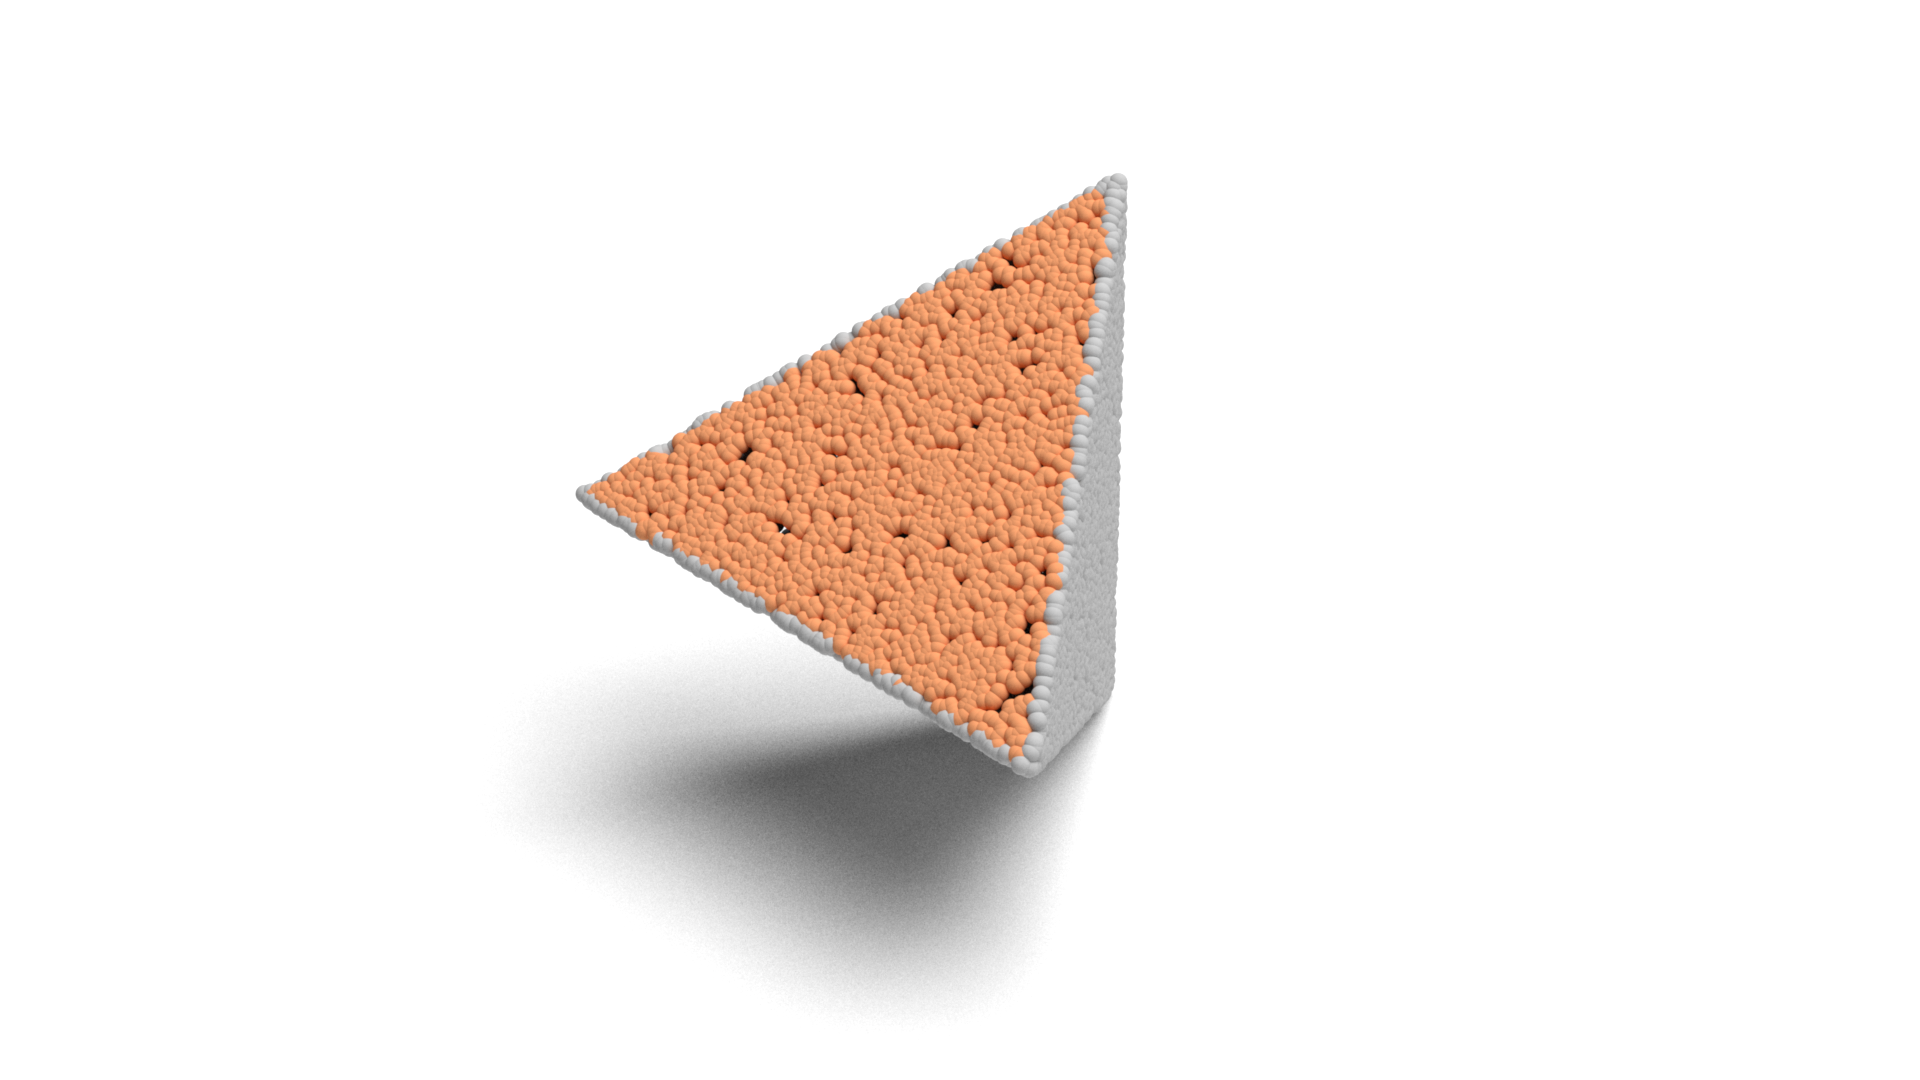}
     % \caption{Cyl-Symsol-I\label{fig:dcyl1}}
     \end{subfigure}%
     \hfill
     \begin{subfigure}{.5\linewidth}
     \centering
     \includegraphics[width=1.\textwidth]{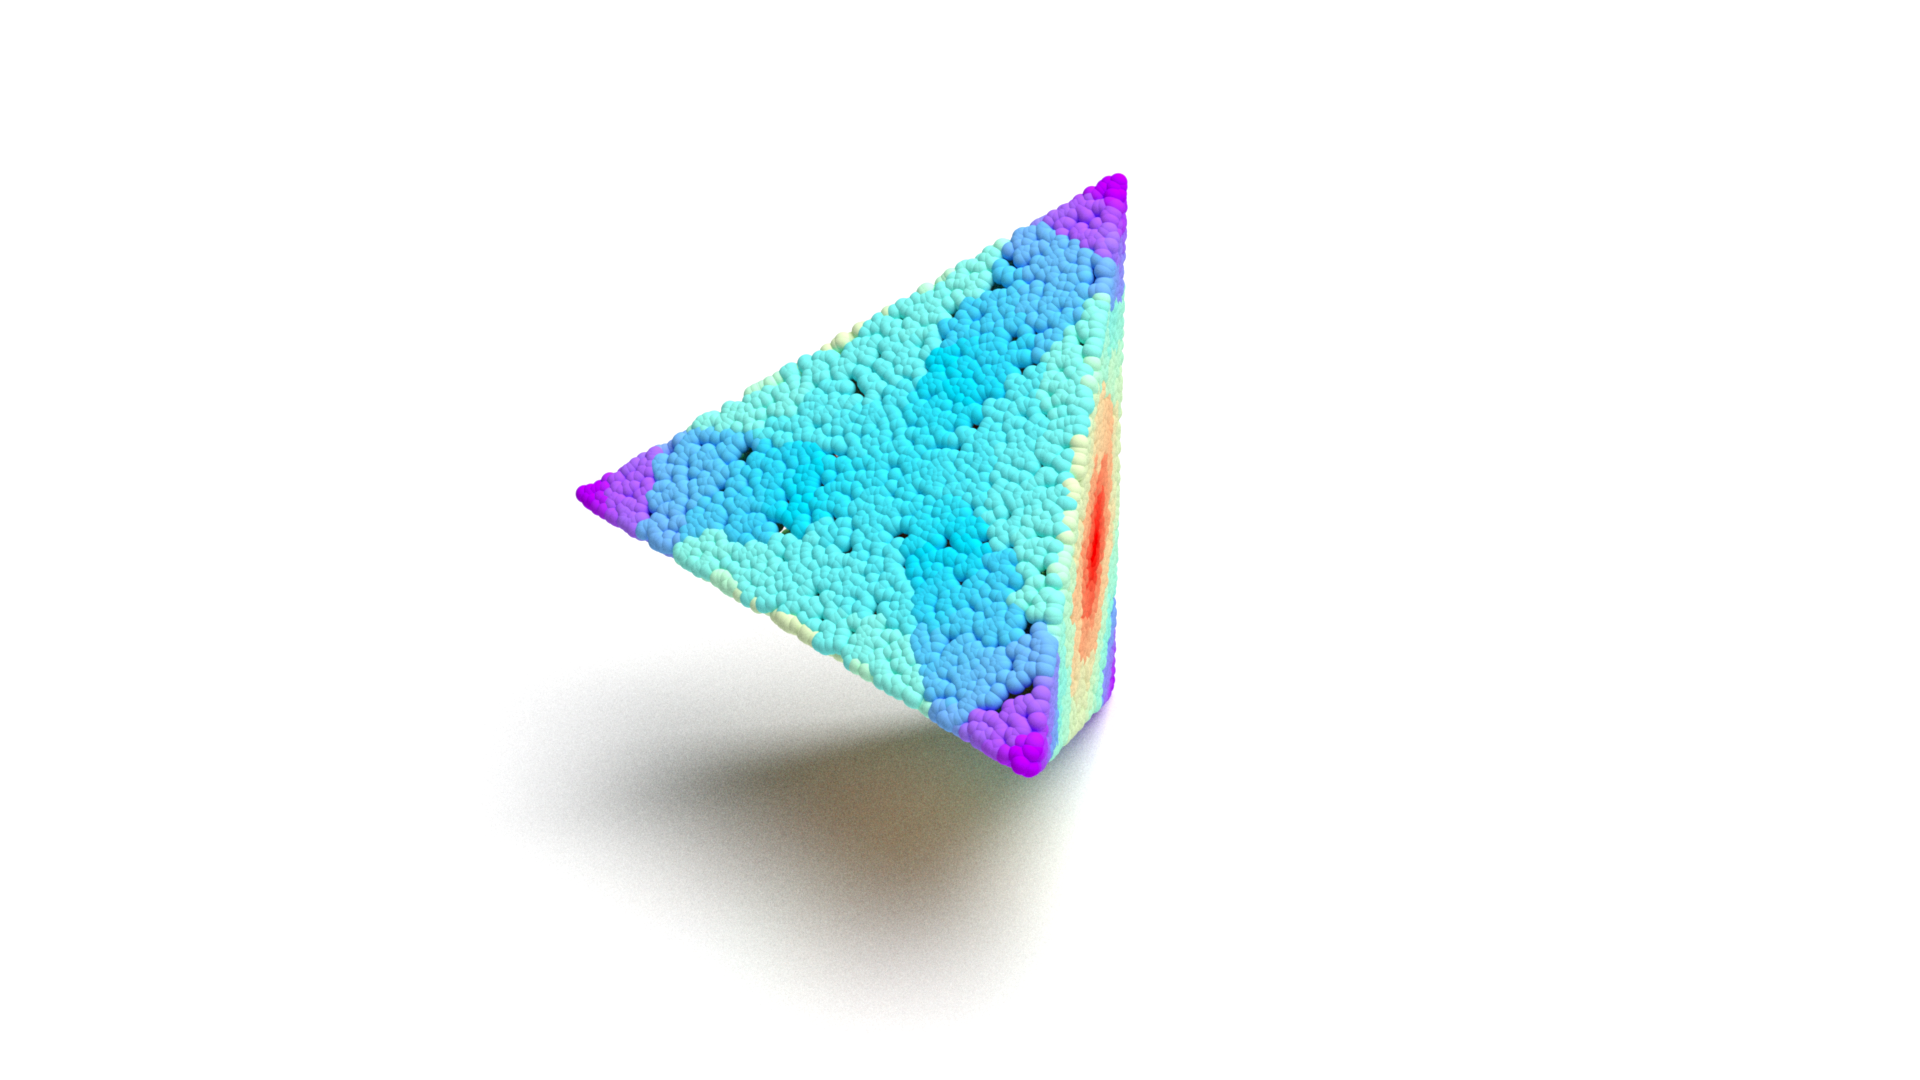}
     % \caption{Cyl-Symsol-I\label{fig:dcyl2}}
     \end{subfigure}%
     \hfill
     \hfill
\\
     \begin{subfigure}{.5\linewidth}
     \centering
     \includegraphics[width=1\textwidth]{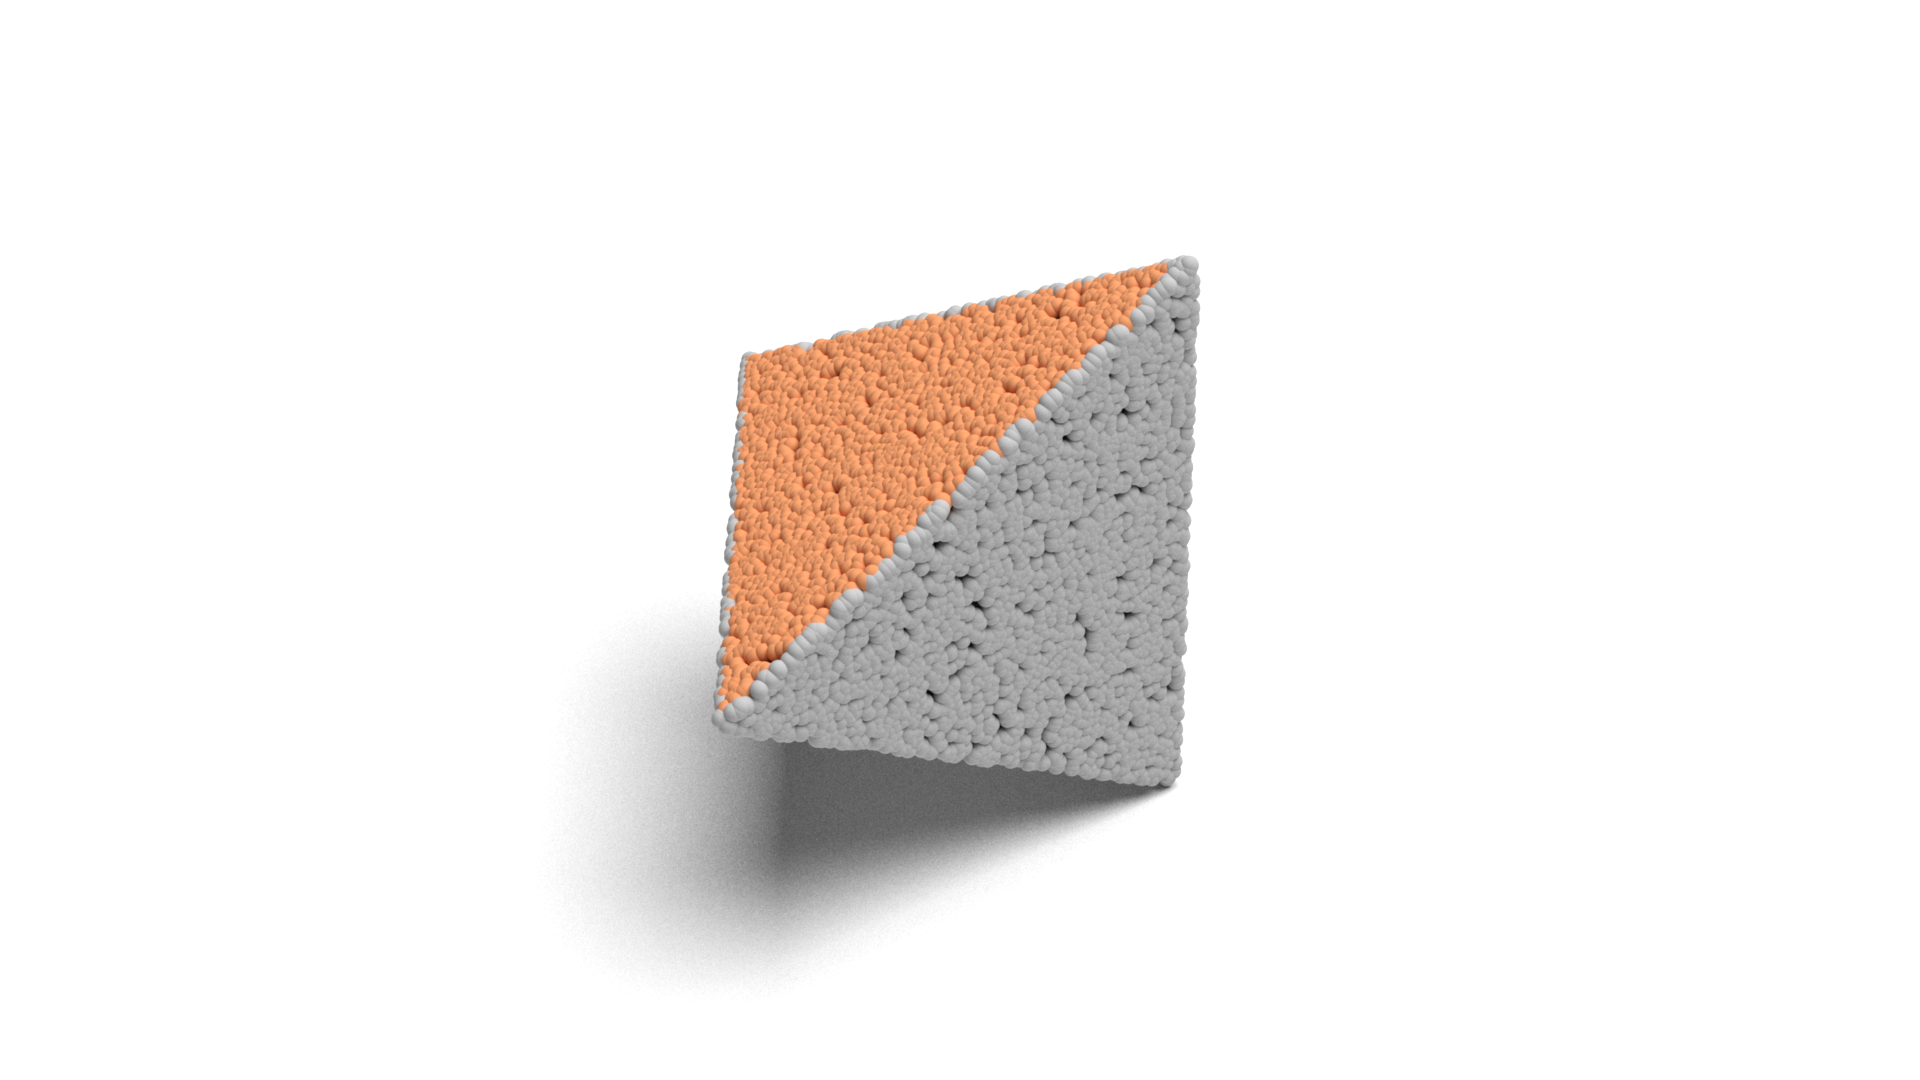}
     % \caption{Cyl-Symsol-I\label{fig:dcyl1}}
     \end{subfigure}%
     \hfill
     \begin{subfigure}{.5\linewidth}
     \centering
     \includegraphics[width=1.\textwidth]{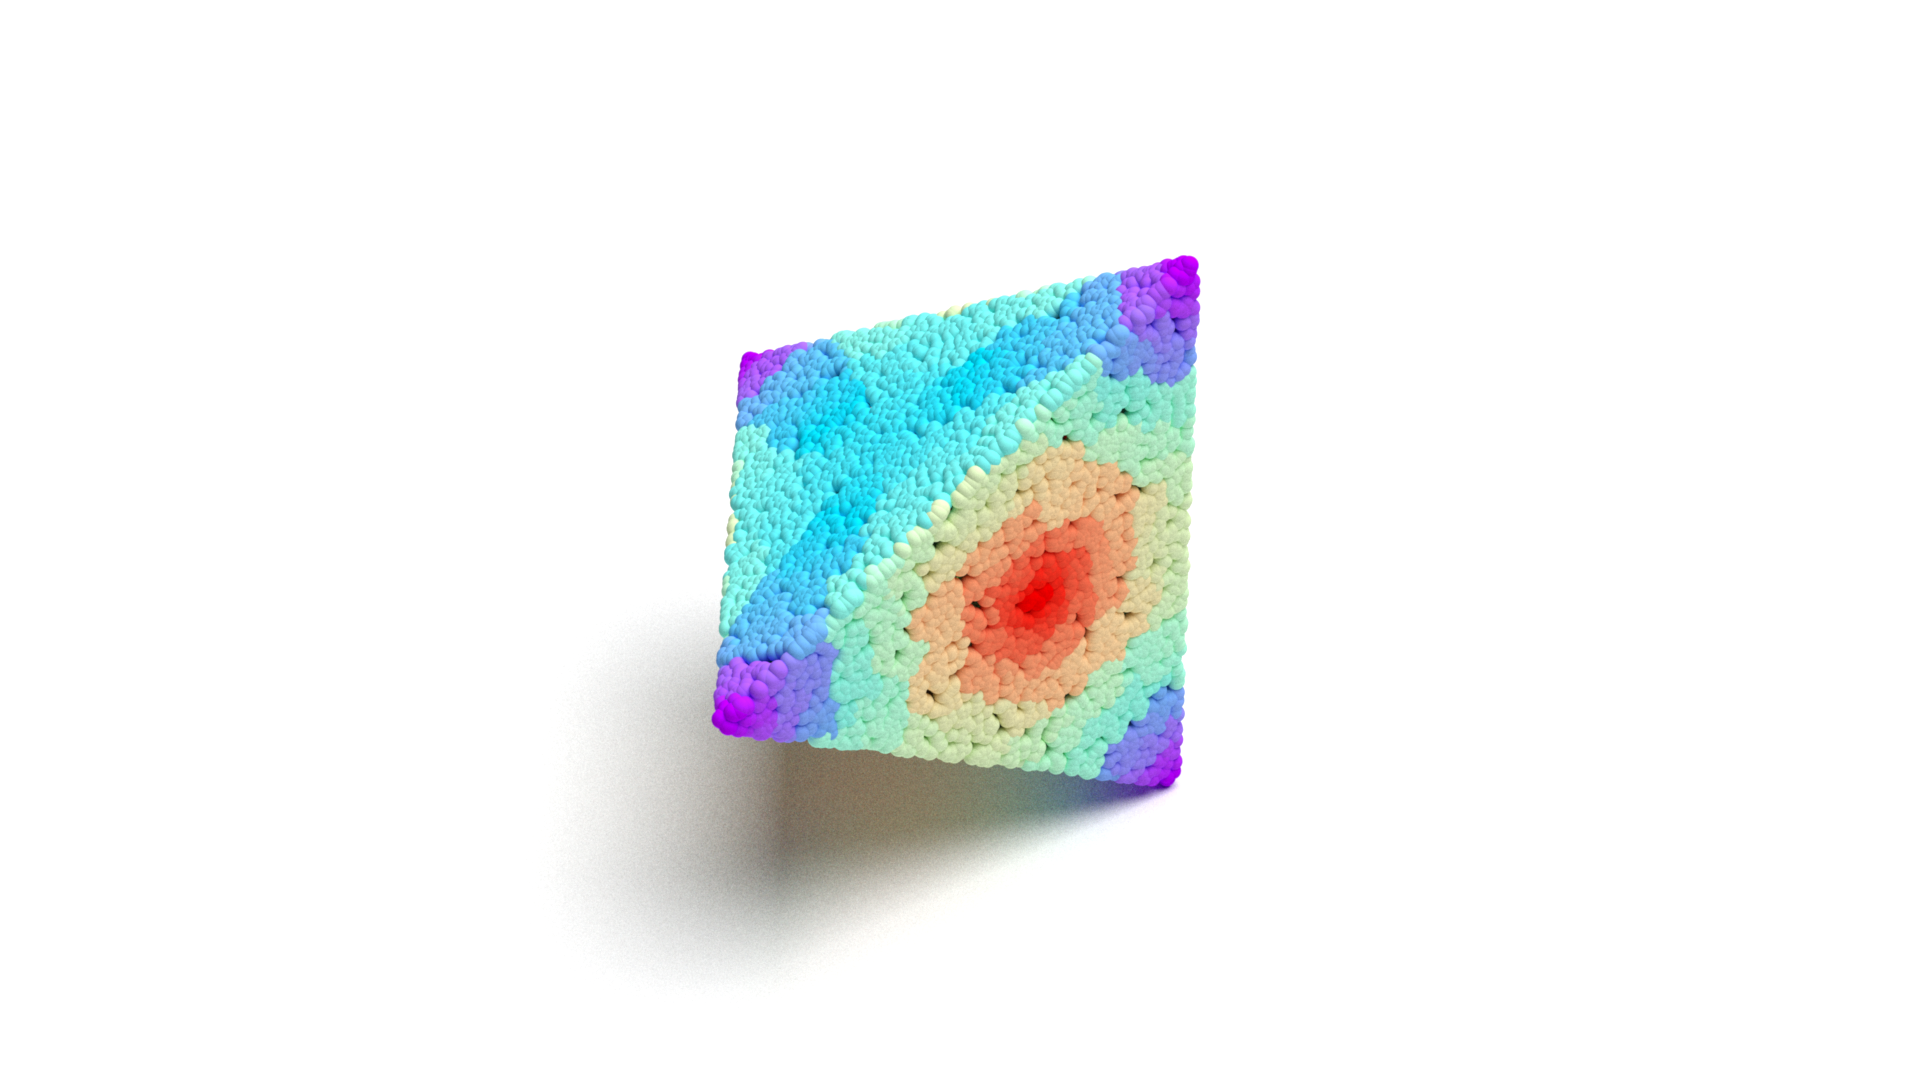}
     % \caption{Cyl-Symsol-I\label{fig:dcyl2}}
     \end{subfigure}%
     \hfill\\
     \begin{subfigure}{.5\linewidth}
     \centering
     \includegraphics[width=1\textwidth]{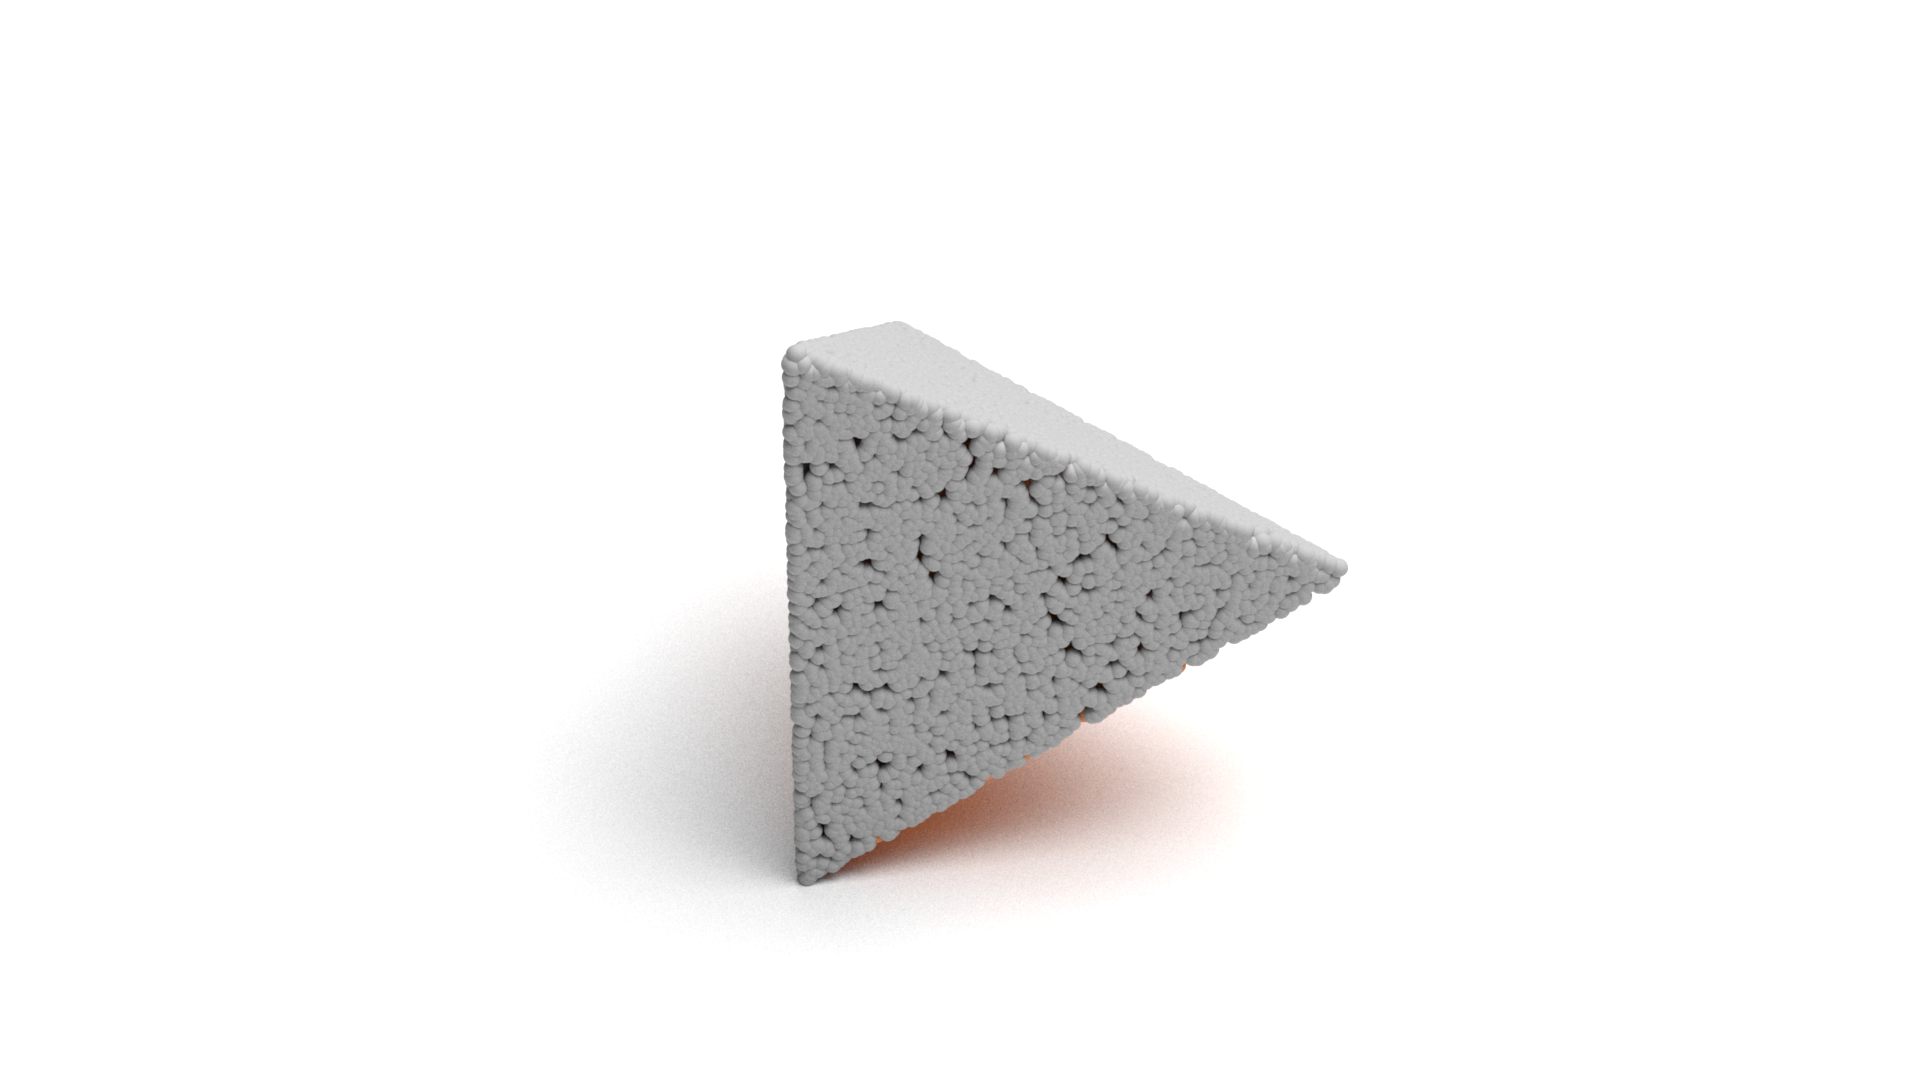}
     % \caption{Cyl-Symsol-I\label{fig:dcyl1}}
     \end{subfigure}%
     \hfill
     \begin{subfigure}{.5\linewidth}
     \centering
     \includegraphics[width=1.\textwidth]{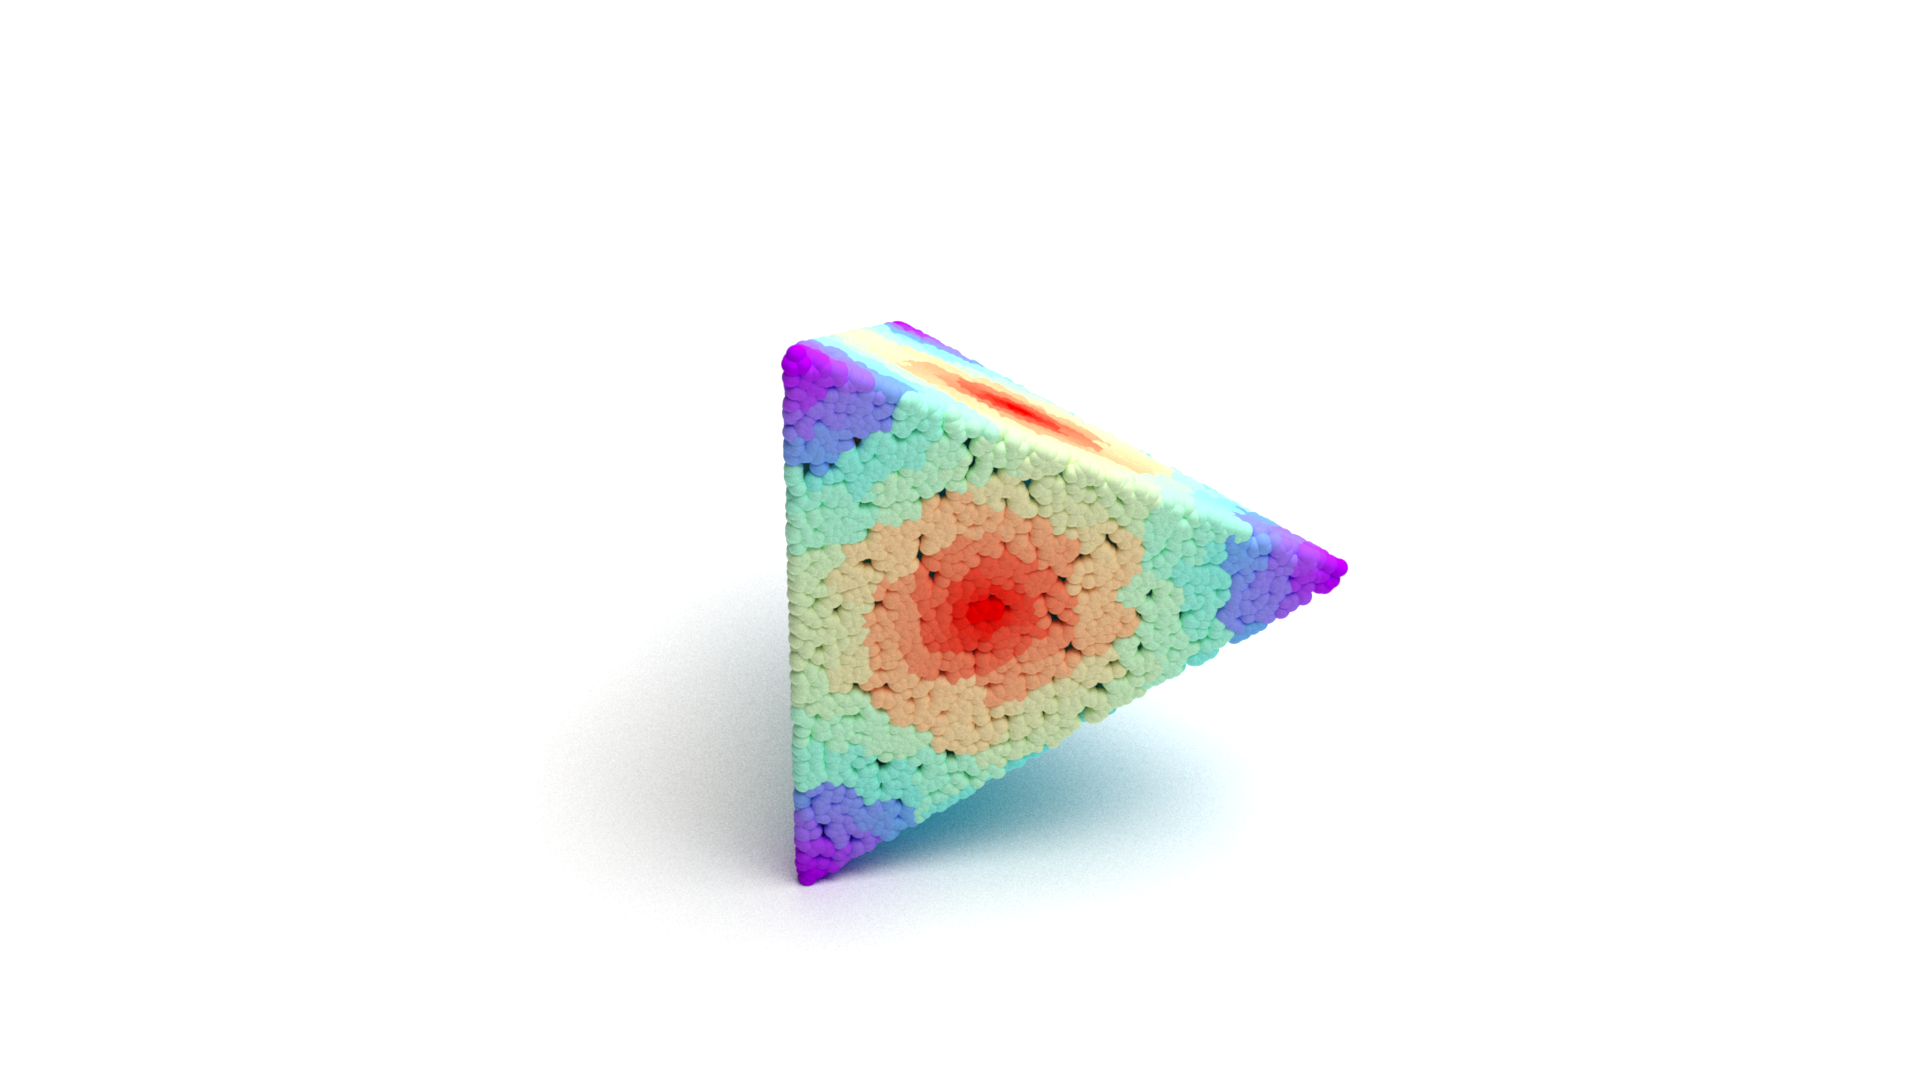}
     % \caption{Cyl-Symsol-I\label{fig:dcyl2}}
     \end{subfigure}%
     \hfill
     \caption{Feature visualization of SurfEmb features for tetX object where a face of tetrahedron is textured with orange color. The first column shows the point cloud from the textured CAD model. The second column shows the per-point feature visualization of the point cloud from different viewpoints. Note that the features are computed in canonical orientation. The visualization indicates different rotations to illustrate the difference in features on the orange face and non-textured faces. The features are clearly different on the non-textured sides compared to the textured side. Also, all of the non-textured sides have similar features.    
     \label{fig:featViz}}
\end{figure}
\begin{figure}
     \centering
     \begin{subfigure}{.3\linewidth}
     \centering
     \includegraphics[width=0.8\textwidth]{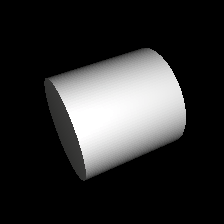}
     % \caption{Cyl-Symsol-I\label{fig:dcyl1}}
     \end{subfigure}%
     \hfill
     \begin{subfigure}{.3\linewidth}
     \centering
     \includegraphics[width=.8\textwidth]{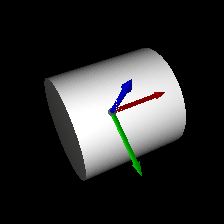}
     % \caption{Cyl-Symsol-I\label{fig:dcyl2}}
     \end{subfigure}%
     \hfill
     \begin{subfigure}{.3\linewidth}
     \centering
     \includegraphics[width=0.8\textwidth]{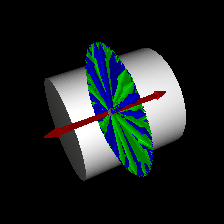}
     % \caption{Cyl-Symsol-I\label{fig:dcyl3}}
     \end{subfigure}%
     \hfill
     \\
     \begin{subfigure}{.3\linewidth}
     \centering
     \includegraphics[width=.8\textwidth]{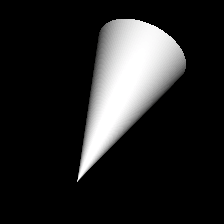}
     % \caption{Tet-Symsol-I\label{fig:tetS1}}
     \end{subfigure}%
     \hfill
     \begin{subfigure}{.3\linewidth}
     \centering
     \includegraphics[width=0.8\textwidth]{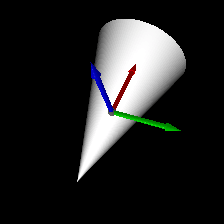}
     % \caption{Tet-Symsol-I\label{fig:tetS2}}
     \end{subfigure}%
     \hfill
     \begin{subfigure}{.3\linewidth}
     \centering
     \includegraphics[width=0.8\textwidth]{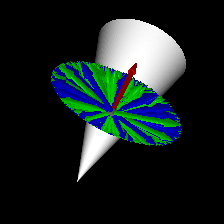}
     % \caption{Tet-Symsol-I\label{fig:tet2S2}}
     \end{subfigure}%
     \hfill
     \\
     \begin{subfigure}{.3\linewidth}
     \centering
     \includegraphics[width=0.8\textwidth]{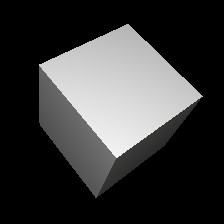}
     % \caption{Cube-Symsol-I\label{fig:tetS1}}
     \end{subfigure}%
     \hfill
     \begin{subfigure}{.3\linewidth}
     \centering
     \includegraphics[width=.8\textwidth]{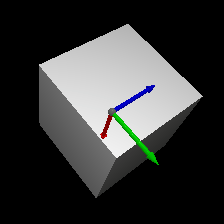}
     % \caption{Cube-Symsol-I\label{fig:tetS2}}
     \end{subfigure}%
     \hfill
     \begin{subfigure}{.3\linewidth}
     \centering
     \includegraphics[width=.8\textwidth]{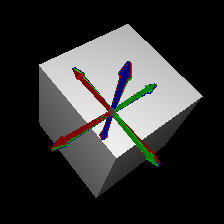}
     % \caption{Cube-Symsol-I\label{fig:tet2S2}}
     \end{subfigure}%
     \hfill
      \\
     \begin{subfigure}{.3\linewidth}
     \centering
     \includegraphics[width=.8\textwidth]{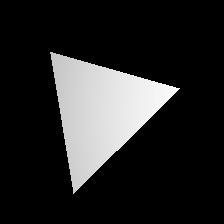}
     % \caption{Cone-Symsol-I\label{fig:tetS1}}
     \end{subfigure}%
     \hfill
     \begin{subfigure}{.3\linewidth}
     \centering
     \includegraphics[width=.8\textwidth]{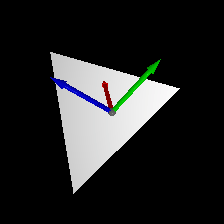}
     % \caption{Cone-Symsol-I\label{fig:tetS2}}
     \end{subfigure}%
     \hfill
     \begin{subfigure}{.3\linewidth}
     \centering
     \includegraphics[width=.8\textwidth]{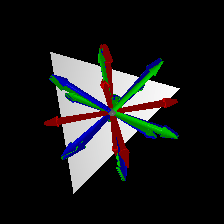}
     % \caption{Cone-Symsol-I\label{fig:tet2S2}}
     \end{subfigure}%
     \hfill
      \\
     \begin{subfigure}{.3\linewidth}
     \centering
     \includegraphics[width=.8\textwidth]{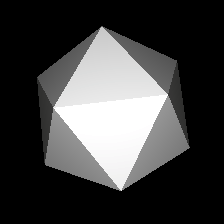}
     % \caption{Cone-Symsol-I\label{fig:tetS1}}
     \end{subfigure}%
     \hfill
     \begin{subfigure}{.3\linewidth}
     \centering
     \includegraphics[width=.8\textwidth]{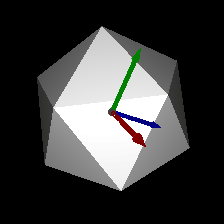}
     % \caption{Cone-Symsol-I\label{fig:tetS2}}
     \end{subfigure}%
     \hfill
     \begin{subfigure}{.3\linewidth}
     \centering
     \includegraphics[width=.8\textwidth]{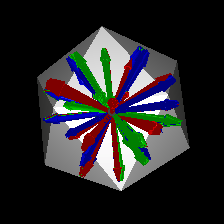}
     % \caption{Cone-Symsol-I\label{fig:tet2S2}}
     \end{subfigure}%
     \hfill
     %  \\
     % \begin{subfigure}{.3\linewidth}
     % \centering
     % \includegraphics[width=1\textwidth]{images/distImages/tet_00126.png}
     % % \caption{Tet-Symsol-I\label{fig:tetS1}}
     % \end{subfigure}%
     % \hfill
     % \begin{subfigure}{.3\linewidth}
     % \centering
     % \includegraphics[width=1.\textwidth]{images/distImages/tet_00736.png}
     % % \caption{Tet-Symsol-I\label{fig:tetS2}}
     % \end{subfigure}%
     % \hfill
     % \begin{subfigure}{.3\linewidth}
     % \centering
     % \includegraphics[width=1\textwidth]{images/distImages/tet_01048.png}
     % % \caption{Tet-Symsol-I\label{fig:tet2S2}}
     % \end{subfigure}%
     % \hfill
     %
         % \includegraphics[width=0.19\textwidth]{sources/images/alignedbadly2.PNG}
      
     \caption{Pose distribution visualization for different objects in Symsol-I. Each row corresponds to a single object starting from a Cylinder, Cone, Cube, Tetrahedron, and Icosa. The first column shows the input image. The second column shows the coordinate reference frame transformed with ground truth rotation and rendered on the input image. In the third column, we transform the coordinate reference frame with top 500 rotations in the distribution and render on the image. Our approach captures the distribution sharply and captures all the modes. This is clearly indicated in cylinder and cone where the red axis is very sharp without much deviation which indicates that the symmetric axis is correctly detected and the variation around the symmetric axis is properly captured in top 500 rotations instead of focusing on some specific modes. The sharpness is also clearly visible in cube, tetrahedron, and icosa where the axes have less blur around them.   
     \label{fig:ourViz}}
\end{figure}

\clearpage

% \section{Rationale}
% \label{sec:rationale}
% % 
% Having the supplementary compiled together with the main paper means that:
% % 
% \begin{itemize}
% \item The supplementary can back-reference sections of the main paper, for example, we can refer to \cref{sec:intro};
% \item The main paper can forward reference sub-sections within the supplementary explicitly (e.g. referring to a particular experiment); 
% \item When submitted to arXiv, the supplementary will already included at the end of the paper.
% \end{itemize}
% % 
% To split the supplementary pages from the main paper, you can use \href{https://support.apple.com/en-ca/guide/preview/prvw11793/mac#:~:text=Delete%20a%20page%20from%20a,or%20choose%20Edit%20%3E%20Delete).}{Preview (on macOS)}, \href{https://www.adobe.com/acrobat/how-to/delete-pages-from-pdf.html#:~:text=Choose%20%E2%80%9CTools%E2%80%9D%20%3E%20%E2%80%9COrganize,or%20pages%20from%20the%20file.}{Adobe Acrobat} (on all OSs), as well as \href{https://superuser.com/questions/517986/is-it-possible-to-delete-some-pages-of-a-pdf-document}{command line tools}.
